# Supplementary material for: Towards Visual Taxonomy Expansion
Source: arXiv:2309.06105 source file (2023-09-12)
Supplement: Supplementary file 1 [file 9-appendix.tex]

\appendix

\section{Chinese Hypernymy Dataset Construction}
\label{appd:dataset}

This section will discuss the details of Chinese hypernymy dataset construction. We construct the dataset on the Meituan platform, which is one of the world's largest life service platforms in China. This platform covers most aspects of our daily life, such as delivery service, food, entertainment, and accommodation.

\subsection{Source Data Preparation}
Meituan is a leading life service platform, maintaining a large scale of taxonomy with almost 600k edges. Thus, we utilize the existing taxonomy as our training set, reducing the labor required for annotation. As for the test set, We choose query-click logs from Meituan. To protect user privacy, we eliminate all user-related information (e.g., user id, username, timestamp, etc) and only leave user-generated queries and clicked corresponding item concepts in the dataset.

In our observation, despite the large scale of the existing taxonomy, 91.67\% of the edges follow the suffix pattern, that is the hyponym ends with the hypernym. For example, Japanese \textit{Ramen} is a kind of \textit{Ramen}, and Vanilla \textit{Latte} is a kind of \textit{Latte}. We define a hypernymy pair with the suffix pattern to contain the suffix hypernymy. Thus, to improve the diversity of taxonomy, we focus on non-suffix hypernymy and remove all suffix hypernymy from our sources.

To collect images for terms, we use images on the Meituan platform. For hyponyms in the training set, we search the term in the Meituan scenario and use the retrieved product image. As for hyponyms in the test set, a clicked item naturally contains an image in the Meituan scenario, which we use as its visual features.

After the above steps, we construct an automatically-labeled training set with 10,697 non-suffix hypernymy pairs and an unlabeled test set with 2,000 pairs of anonymous query-click logs.

\subsection{Annotation}
Annotators are required to annotate whether given pairs in the test set are hypernymy pairs. We ask three separate annotators to annotate the test set. These annotators are workers from Meituan and have been paid adequately for their annotation work. All three annotators are from China.

Moreover, we write detailed instructions on what hypernymy relation is and list several types of non-hypernymy relations. For example, we divide non-hypernymy relations in query-click logs into three types: 1) synonymy, 2) unrelated relations, and 3) ``prototypical hypernym''. Especially, we give detailed explanations of ``prototypical hypernym''.

\subsection{Details}
In our Chinese hypernymy dataset, the training set consists of 10,697 pairs of non-suffix hypernymy with 7,192 different hyponyms and 4,372 hypernyms. And the test set contains 1217 positive pairs and 783 negative pairs. To estimate the overall quality of the dataset, two authors of this paper annotate 200 randomly selected hypernymy pairs. The result shows that the precision and recall are 98.65\% and 97.31\%.

\section{Parameter Settings}
For our model implementation, we use ``bert-base-uncased''\footnote{https://huggingface.co/bert-base-uncased} and ``bert-base-chinese''\footnote{https://huggingface.co/bert-base-chinese} as the textual backbone and ``resnet-101''\footnote{https://huggingface.co/microsoft/resnet-101} as the visual backbone. These pre-trained models are under the license of ``apache-2.0'' which allows us to use them for academic purposes. And they are originally to serve as encoders for downstream tasks.
For the prototype embedding table, we set $k=1024$ and $e=256$. For temperatures hyper-parameter in contrastive learning, we set $\tau_{text}=0.1$, $\tau_{proto}=0.1$. For EMA, we set $\alpha=0.999$ and $\epsilon=0.001$. Apart from prototypes, other parameters are optimized by Adam \citep{https://doi.org/10.48550/arxiv.1412.6980} with a learning rate of 5e-5. We train our model (parameter number of approximately 150M) on one NVIDIA Tesla A100 GPU with a fixed batch size of 128 in approximately 12 hours.
